# Supplementary material for: Entanglement Entropy and Algebra in Quantum Field Theory
Source: arXiv:2307.06286 source file (2023-07-12)
Supplement: Supplementary file 1 [file 21Appendix.tex]

\appendix
\chapter{Extra Information}
Some more text ...
